# Supplementary material for: Logistic regression models: practical induced prior specification
Source: arXiv:2501.18106 source file (2025-02-02)
Supplement: Supplementary file 1 [file AppendixB_Generating_Functions.tex]

\appendix 
\section{Logistic Distribution and Generating
Functions}

\subsubsection{MGF and CF for Logistic Distribution}
Generating functions of random variables 
are the expected value of a specific transformation
of a random variable, e.g., $E_X[\exp(tX)]$ =
$\int \exp(tx) p(x) dx$.
Knowledge of the generating function can sometimes
be used to learn about or sample from the underlying
probability distribution, $p(x)$. Here we show
two generating functions for the logistic distribution
that are of potential use for learning about
the prior distribution for logistic regression 
coefficients which induces a Logistic(0,1) distribution
on the logit of $\theta$, and thereby induces a
Uniform(0,1) distribution on the Bernoulli parameter
$\theta$.

The moment generating function (MGF) and characteristic function (CF) for the logistic distribution are the
following.
\begin{align}
\label{eq:MGM.logistic.general}
MGF(X) = E[\exp(tX)] &= \exp(\mu t)
\frac{ \Gamma(1-st) \Gamma(1+st)}{\Gamma(2)}, ~~ -\frac{1}{s} < t < \frac{1}{s} \\
CF(X) = E[\exp(itX)] &= \exp(i t \mu) 
   \frac{\pi s t}{\sinh(\pi s t)}  
 =  \frac{\exp(i t \mu)* 2 * \pi s t}{\exp(\pi s t) - \exp(-\pi s t)}
\end{align}
 In the special case Logistic($\mu=0$, $s=1$),
\begin{align} 
\label{eq:MGF.logistic}
MGF(\beta) &=  \frac{\Gamma(1-t) \Gamma(1+t)}{\Gamma(2)}
, ~~ -1 < t < 1 \\
\label{eq:CF.logistic}
 CF(\beta) &
 =  \frac{2 \pi t}{\exp(\pi t) - \exp(-\pi t)}
 \end{align}
 Given knowledge of the characteristic function
 of a pdf, there are numerical procedures for
 inverting characteristic functions to calculate,
 at least numerically, and occasionally
 analytically $\Pr(a < X <b)$ from the underlying
 pdf $p$ which ``generated'' the CF\footnote{See Theorem
 107 in https://sas.uwaterloo.ca/~dlmcleis/s901/chapt6.pdf}.

 \paragraph{Side notes.}
 \begin{enumerate}
\item MGFs do not always exist, i.e., the integral may
 be divergent (not finite), but when they do, they can be used to find the moments of a random variable---assuming the moments
exist. To find the $n^{th}$
moment, the $n^{th}$ derivative of the MGF with respect to
the parameter $t$ is calculated
and evaluated at $t$=0.  For example, for an absolutely
continuous random variable (with density function $f(x)$), the 1st moment is:
\begin{align*}
\frac{d}{dt} MGF(x)|_{t=0} &= \frac{d}{dt} \int \exp(tx) f(x) dx|_{t=0}
= \int \frac{d}{dt}\exp(tx) f(x) dx|_{t=0} =
\int x f(x) dx = E[X]
\end{align*}
where Leibniz integral rule\footnote{https://en.wikipedia.org/wiki/Leibniz\_integral\_rule} allows the differentiation
to pass to the inside of the integral.
%----
\item CFs (for real valued random variables) always exist ``since it is an integral of a bounded continuous function over a space whose measure is finite.\footnote{https://en.wikipedia.org/wiki/Characteristic\_function\_(probability\_theory))}''.  As for the MGF, assuming the
moments exist, the moments can be found by differentiating
the CF with respect to the parameter $t$ with an additional
step to ``remove'' the imaginary unit $i$.

 \end{enumerate}

 %-------------------------------------
\subsubsection{\label{subsub:MGF.Logistic} \tcr{Aside \#1: using Logistic MGF
to calculate moments}}  Partly as an exercise
and partly for reasons to be discussed later,
here I am trying to use the MGF for the
logistic calculate the expected value ($\mu$).  Thus, I want to calculate $\frac{dMGF(t)}{dt}$ and evaluate it at $t$=0.
\tcb{However, the following calculation of the first derivative
of the MGF does not appear to be correct. Now corrected :-)} 
\begin{align*}
 \frac{dMGF(t)}{dt} & = \frac{d}{dt} \exp(\mu t) \frac{\Gamma(1-st) \Gamma(1+st)}{\Gamma(2)} \\
% &=\mu\exp(\mu t) \frac{\Gamma(1-st) \Gamma(1+st)}{\Gamma(2)}  + \\
% & ~~ \frac{\exp(\mu t)}{\Gamma(2)} 
% \left [ \Gamma(1-st) \psi(1-st) \Gamma(1+st) +
%        \Gamma(1-st) \Gamma(1+st) \psi(1+st)\right ] \\
& = \frac{\mu\exp(\mu t)}{\Gamma(2)} \left[\Gamma(1-st)s\Gamma'(1+st) - s\Gamma'(1-st)\Gamma(1+st)\right]
\end{align*}
%where $\psi(Z)$ is the digamma function.  The above is using the fact that $\psi(Z)$ is the derivative of $\ln(\Gamma(Z))$, $\frac{d}{dZ}\ln(\Gamma(Z))$ = $\frac{1}{\Gamma(Z)} \frac{d}{dZ} \Gamma(Z)$.

%However there is something wrong with the above derivation.  Letting $t$=0, which should yield $\mu$ actually yields:
%\begin{align*}
%\frac{dMGF(t)}{dt}_{|t=0} &= 
%\mu \frac{\Gamma(1)\Gamma(1)}{\Gamma(2)} +
%\frac{1}{\Gamma(2)} \left [ \Gamma(1) \psi(1) \Gamma(1) +
%        \Gamma(1) \Gamma(1) \psi(1)\right ] \\
%        &= \mu + 2*\psi(1) = \mu -1.154431 
%\end{align*}

Letting $t=0$, in order to derive $\mu$, we have,
\begin{eqnarray*}
    \left. \frac{dMGF(t)}{dt}\right|_{t=0}  & = & \frac{1}{\Gamma(2)} \times [\Gamma(1)s\Gamma'(1) - s\Gamma'(1)\Gamma(1)] = 0.
\end{eqnarray*}
Note that $\Gamma'(1) = \gamma$, referred to as Euler-Mascheroni constant. 

%\tcb{I suspect that there is something ``subtle'' that needs to be done with the analytic calculation of the derivative of this function of $t$. I base this partly on the result I found below.}

According to https://proofwiki.org/wiki/Moment\_Generating\_Function\_of\_Logistic\_Distribution the first derivative is
\begin{align*}
\frac{dMGF(t)}{dt} & = \exp(\mu t) \left [
\mu \int_{\rightarrow 0}^{\rightarrow 1}
\left ( \frac{1-u}{u} \right )^{-st} du
 - s \int_{\rightarrow 0}^{\rightarrow 1}
 \ln \left ( \frac{1-u}{u} \right ) 
 \left ( \frac{1-u}{u} \right )^{-st}
 du 
\right ]
\end{align*}
and a numerical check indicates that the above does
yield the expected value.
\begin{verbatim}
theory.diff.MGF <- function(t,mu,s,delta=0.1) {
  integrand1 <- function(u,t,s) {
    ((1-u)/u)^(-s*t)
  }
  integrand2 <- function(u,t,s) {
    log((1-u)/u)*((1-u)/u)^(-s*t)
  }
  
  p1 <- exp(t*mu)
  p2 <- mu*integrate(f=integrand1,lower=delta,
                     upper=1-delta,t=t,s=s)$value
  p3 <- s*integrate(f=integrand2,lower=delta,
                    upper=1-delta,t=t,s=s)$value
  out <- p1*(p2-p3)
  return(out)
}
theory.diff.MGF(t=0,mu=7,s=3,delta=0.0001)
## [1] 6.9986
\end{verbatim}

Below is a crude numerical calculation of the derivative
of the MGF
\begin{verbatim}
logistic.MGF.deriv.numerical <- function(t,mu,s,delta=0.01) {
  logistic.MGF <- function(t,mu,s) {
    out <- exp(mu*t)*beta(1-t*s,1+t*s)
  return(out)
  }
  numerator <- logistic.MGF(t=t+delta,mu=mu,s=s) - logistic.MGF(t=t,mu=mu,s=s)
  out <- numerator/delta
  return(out)
}
\end{verbatim}

I am not confident that the above numerical calculations
are that ``good'' as the first one tends to overestimate
and the second one tends to underestimate. For example,
\begin{verbatim}
t.val  <- 0; mu.val <- 5; s.val  <- 3
numerical <- logistic.MGF.deriv.numerical(t=t.val,mu=mu.val,s=s.val,delta=0.0001)
theoretical <- logistic.MGF.deriv.theory2(t=t.val,mu=mu.val,s=s.val,delta=0.0001)
cat("Use of MGF: mu=",mu.val,"Numerical=",numerical,"Theoretical=",theoretical,"\n")
## Use of MGF: mu= 5 Numerical= 5.002731 Theoretical= 4.999    
\end{verbatim}

\subsubsection{\label{subsubsec:LaplaceTransform}Laplace transform}
%----
 Another generating function, ``transform'', is
the Laplace transform.  This is of particular interest
to us as procedures for ``recovering'' a probability
density from a Laplace transformation can be more useful
than such procedures based on MGFs or CFs.
This ``inversion'' is discussed more in Section
\ref{subsubsec:HalfLogistic}.
The Laplace transform  is defined for functions
with non-negative domain:
\begin{align*}
\mathcal{L}\{f \}(t) &= \int_0^\infty \exp(-tx) f(x) dx
\end{align*}
where $t$ is a complex number.  When the Laplace transform
exists (integral is not divergent) and the $n^{th}$ moment
exists, the moment can be calculated by differentiation
with respect to $t$ with an additional step of ``removing''
the negative multiplier. For example,
\begin{align*}
\frac{d}{dt} \mathcal{L}\{f \}(t)|_{t=0} &= \frac{d}{dt} \int \exp(-tx) f(x) dx|_{t=0}
= \int \frac{d}{dt}\exp(-tx) f(x) dx|_{t=0} =
\int -x f(x) dx = -E[X]
\end{align*}

When the random variable includes negative values, there
is the two-sided Laplace transform:
\begin{align*}
\mathcal{B}\{f \}(t) & = \int_{-\infty}^\infty \exp(-tx) f(x) dx
\end{align*}
which exists only when the integrals below and
above zero exist:
\begin{align*}
\int_{-\infty}^0 \exp(-tx) f(x) dx < \infty, ~~ & ~~
\int_0^{\infty} \exp(-tx) f(x) dx  < \infty
\end{align*}
Thus $\mathcal{B}\{f \}(t)$ is the MGF with the parameter $-t$ instead
of $t$ and it again can be used to find moments when
they exist. 

However, based on an online integral calculator, $\mathcal{B}\{f \}(t)$ does not exist for the Logistic distribution,
i.e., the integral is divergent.  In particular the
integral below zero is divergent.  However, the integral
above zero does appear to exist, at least for some example cases:
\begin{align*}
\mbox{Logistic}(\mu=3,s=5, t=0.1) &: 
\int_{3}^\infty \exp(-0.1 X) 
\frac{\left ( -\frac{(x-3)}{5} \right ) }
{5 \left ( 1+\exp \left ( -\frac{(x-3)}{5}\right )
\right )^2} \approx 0.336986 
\end{align*}

 \subsubsection{\label{subsubsec:HalfLogistic}Half-Logistic Distribution and the Laplace Transform}
 As mentioned above the
 Laplace Transform has proven useful for 
 inversion to yield samples from the underlying
 pdf \citep{2009_Ridout,2017_Walker}. As also
 noted above, the Laplace transformation
 is only defined for functions with positive support,
 thus ruling out the Logistic distribution. 
 While for random variables with negative values,
 there is the  two-sided Laplace Transform, it does
 not exist for the Logistic distribution because
 the integral over the negative values is divergent.
 
 However given that the integral does converge
 for positive values and that the Logistic distribution
 is symmetric about $\mu$, a workaround is to define a 
 ``half'' Logistic distribution: the logistic restricted 
 to values
 above the location parameter $\mu$ with the following
 pdf:
 \begin{align}
    \label{eq:half.Logistic.pdf}
 \mbox{Half-Logistic}(x; \mu, s) & = 2 
 \frac{\exp \left ( -\frac{(x-\mu)}{s} \right )}
{s \left ( 1+\exp \left ( -\frac{(x-\mu)}{s}\right )
\right )^2}, ~~~~ x \ge \mu 
 \end{align}
 
 Some remarks:
 \begin{itemize}
     \item The Half-Logistic is a proper 
 pdf as it integrates to 1 over $x \ge \mu$,
 \begin{align}
    2 \int_{\mu}^\infty 
     \frac{\exp \left ( -\frac{(x-\mu)}{s} \right )}
{s \left ( 1+\exp \left ( -\frac{(x-\mu)}{s}\right )
\right )^2} dx & = 1
 \end{align}.
  \item The expected value is
 not defined, i.e., the integral diverges. This
 implies that the MGF is not defined as $\exp(tx)$ $>$ $x$
 for $t>0$.
 \item The Laplace transform does appear to
 be defined for the half Logistic
 \begin{align}
 \label{eq:Half.Logistic.Laplace.Transform}
    E[\exp(-tX)] &= 2 \int_0^\infty \exp(-tx) 
       \frac{\exp \left ( -\frac{x}{s} \right )}
{s \left ( 1+\exp \left ( -\frac{x}{s}\right )
\right )^2} dx ~~~~  < \infty?
 \end{align}
 This tentative conclusion is  based on several
 example trials using an online integral 
 calculator \footnote{https://www.integral-calculator.com/}.
 Referring to the example given previously:
\begin{align*}
\mbox{Half-Logistic}(\mu=3,s=5, t=0.1) &: 
2 \int_{3}^\infty \exp(-0.1 x) 
\frac{\left ( -\frac{(x-3)}{5} \right ) }
{5 \left ( 1+\exp \left ( -\frac{(x-3)}{5}\right )
\right )^2} \approx 0.673972 
\end{align*}
However, we have not found an analytic formula.
 \item If a sample value can be simulated from the 
 Half-Logistic, denoted $x$,
 then samples can easily drawn from the full Logistic
 by changing the value to $x^*$=$\mu-x$, with probability 0.5.  
 
 \end{itemize}
