# Supplementary material for: Logistic regression models: practical induced prior specification
Source: arXiv:2501.18106 source file (2025-02-02)
Supplement: Supplementary file 2 [file AppendixC_Using_GeneratingFunctions_to_define_Priors.tex]

\section{\label{sec:full.prior.determination}$\pi(\beta)$ determination using generating functions} 
Here we consider what might be done to specify
full prior distributions for the $\beta$'s, not just
their mean and variance, that would match (or
well approximate) the Logistic(0,1).  Our approach is 
based on generating functions.

To begin we review a well-known result regarding 
moment generating functions (MGFs) for sums of 
independent random variables, i.e., convolutions. 
Let $X$ and $Y$ be independent random variables that have MGFs, MGF($X$) and MGF($Y$) and define $Z$ = $X+Y$, then
\begin{align*}
  MGF(Z) = E[\exp(tZ)] & = E[\exp(t(X+Y))] =
E[\exp(tX)] E[\exp(tY)] = MGF(X)*MGF(Y)
\end{align*} 
The same holds for characteristic functions (CFs)
\begin{align*}
  CF(Z) = E[\exp(itZ)] & = E[\exp(it(X+Y))] =
E[\exp(itX)] E[\exp(itY)] = CF(X)*CF(Y)
\end{align*} 
This result is sometimes used to determine if the
probability distribution for a sum of independent
random variables with known MGFs are such that
the resulting MGF is from a recognizable probability distribution.
For example, if $X$ and $Y$ are independent Poisson
random variables with rate parameters $\lambda_1$ and
$\lambda_2$,
\begin{align*}
 MGF(Z) & = MGF(X)*MGF(Y) = e^{\lambda_1(e^{t}-1)}
 e^{\lambda_2(e^{t}-1)} = e^{(\lambda_1+\lambda_2)(e^{t}-1)}
\end{align*}
where the last term is the MGF for a Poisson($\lambda_1+\lambda_2$).

\subsection{Linear model without covariates, or
 all $x_i$=1}
We now return to the simplistic GLM, where $\eta$ is 
either the sum of
$p+1$ iid variables, or equivalently it is the usual linear
combination of covariates but all are equal to 1.
We assume, to solve the many-to-one problem,
that the priors for the $\beta_i$'s are all the same and independent ($\beta_i$'s are iid). Then
\begin{align}
\label{eq:MGF.eta}
MGF(\eta) &= MGF(\beta_0 + \sum_{i=1}^p \beta_i) 
= \prod_{i=0}^p MGF(\beta_i) = 
\left [ MGF (\beta) \right ]^{p+1}
\end{align}
Thus the MGF for $\beta$ needs to be the $(1+p)^{th}$
root of the MGF for $\eta$. If the distribution for
$\eta$ is Logistic($\mu$, $s$), then  
\begin{align}
\label{eq:MGF.logistic.eta}
    MGF(\beta)   & = 
    \begin{cases}
\left [ \exp(\mu t) \frac{\Gamma(1-st) \Gamma(1+st)}{\Gamma(2)}
\right ]^{\frac{1}{p+1}} & \mbox{arbitrary $\mu$, $s$},  ~~ -\frac{1}{s} < t < \frac{1}{s} \\
    \left [ \frac{\Gamma(1-t) \Gamma(1+t)) )}{\Gamma(2)}
  \right ]^{\frac{1}{p+1}} & \mu=0, s=1,  ~~ -1 < t < 1
  \end{cases}
\end{align}
Figure \ref{F:Shrunk_MGF} shows how the shape
of the ``shrunk'' MGF widens with increasing $p$.
\begin{figure}[h]
    \centering
    \includegraphics{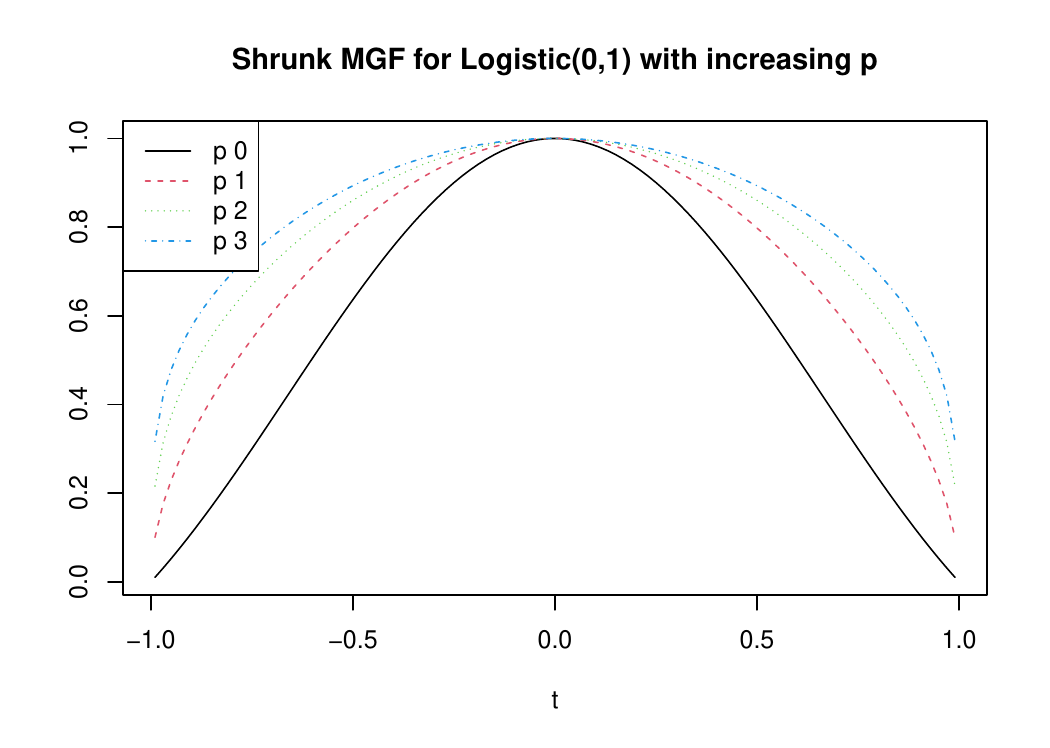}
    \caption{MGF$^{1/(1+p)}$ for Logistic(0,1).}
    \label{F:Shrunk_MGF}
\end{figure}

For CFs:
\begin{align}
\label{eq:CF.logistic.eta}
    CF(\beta)   & = 
    \begin{cases}
\left [  \frac{\exp(i t \mu)* 2 * \pi s t}
{\exp(\pi s t) - \exp(-\pi s t)}
\right ]^{\frac{1}{p+1}} & \mbox{arbitrary $\mu$, $s$} \\
\left [  \frac{  2 * \pi  t}
{\exp(\pi t) - \exp(-\pi  t)}
\right ]^{\frac{1}{p+1}} &    \mu=0, s=1
  \end{cases}
\end{align}

\subsubsection{\tcb{Laplace Transform}}
\tcb{The Laplace Transform, when it exists, has the
same property regarding convolutions as the MGF
and the CF:
\begin{align}
\mathcal{L}\{ g(\eta) \}(t) &=
\prod_{i=0}^p \mathcal{L} \{ g(\beta_i)   \} (t) 
= [\mathcal{L} \{ g(\beta)   \} (t) ]^{p+1}
\end{align}
In particular we want $\eta$ to have a 
Logistic($\mu=0$, $s=1$) distribution. However, the
Logistic does not have a (two-sided) Laplace Transform. 
A random variable that is Half-Logistic does have
a Laplace Transform.  If $Y$ is Half-Logistic then
 $X \times Y$, where $X$ is a random variable
with values -1 and +1 occurring with probability 0.5
that is independent of $Y$, is Logistic. 
Thus define $\eta$=$XY$, and write $XY$ as the sum
of $p+1$ iid random variables:
\begin{align*}
    XY = \eta &=   \sum_{i=0}^p \beta_i,
    ~~ \Rightarrow \\
Y &= \frac{1}{X}     \sum_{i=0}^p \beta_i = X    \sum_{i=0}^p \beta_i  
\end{align*}
where the last equality holds because $X$ = $1/X$ are
identical. 
Can one work with the Laplace Transform of $Y$, using
eq'n (\ref{eq:Half.Logistic.Laplace.Transform}), and determine what the Laplace Transform for $\beta$ should
be given knowledge of the distribution of $X$? 
\begin{align}
\label{eq:link.eta.Half.Logistic}
E_Y[\exp(-tY)] &= E_{\beta_0,\ldots,\beta_p} \left [ \exp \left (-t X    \sum_{i=0}^p \beta_i \right )     \right ]
\end{align}
where the lefthand side  equals eq'n
(\ref{eq:Half.Logistic.Laplace.Transform}).
If condition the righthand side on $X$, thus fixing
its value, one could view each term in the exponential
at a Laplace Transform with respect to $tX$:
\begin{align}
\label{eq:link.eta.Half.Logistic.part2}
E_Y[\exp(-tY)] &= E_X \left [\left ( E_{\beta} 
\left ( \exp(-tX \beta)\right ) \right )^{p+1}
 | X \right ]
\end{align}
}

%-------------------------------------
\subsubsection{\label{subsub:MGF.beta} \tcr{Aside \#2: using the MGF for
$\beta$ to calculate moments}} 
As for Section \ref{subsub:MGF.Logistic},
one ``should'' be able to use the MGF for $\beta$, eq'n
\ref{eq:MGF.logistic},  to find the
moments of $\beta$.  In particular,
\begin{align*}
    \left. \frac{dMGF(\beta)}{d\beta}\right|_{\beta=0} & = E[\beta] \\
     \left. \frac{dMGF(\beta)^2}{d^2\beta}\right|_{\beta=0} &= E[\beta^2]
\end{align*}
\tcb{However, given that I'm apparently doing something
wrong with the simpler logistic MGF, the following
working through of the first derivative is wrong}:

{\small 
\begin{align*}
 \frac{dMGF(\beta)}{d\beta} & = 
 \frac{1}{p+1} \left [ \exp(\mu t)  
 \frac{\Gamma(1-st) \Gamma(1+st)}{\Gamma(2)}
\right ]^{-\frac{p}{p+1}} \times \\
& ~~  \left [ \mu \exp(\mu t) 
 \frac{\Gamma(1-st) \Gamma(1+st)}{\Gamma(2)}  
 \right . 
 \\
 & ~~ +
\left .  \exp(\mu t) 
 \frac{\Gamma(1-st)\psi(1-st)\Gamma(1+st) 
+ \Gamma(1-st)\Gamma(1+st)\psi(1+st)}{\Gamma(2)} \right ] 
\end{align*} }

where $\psi(Z)$ is the \textit{digamma} function.

\tcb{Work through similarly to corrected logistic derivation}

\begin{eqnarray*}
\frac{dMGF(\beta)}{dt} & = & \frac{1}{p+1} \left[\exp(\mu t) \frac{\Gamma(1-st)\Gamma(1+st)}{\Gamma(2)}\right] ^{- \frac{p}{p+1}} \\
& & \quad \times \frac{\mu\exp(\mu t)}{\Gamma(2)} \left[\Gamma(1-st)s\Gamma'(1+st) - s\Gamma'(1-st)\Gamma(1+st)\right]
\end{eqnarray*}

So that 
\begin{eqnarray*}
\left. \frac{dMGF(\beta)}{dt} \right|_{t=0} & = & 
\frac{1}{p+1} \Gamma(2)^{\frac{p}{p+1}} \times \frac{\mu}{\Gamma(2)} \times 0 = \frac{1}{p+1} \Gamma(2)^{p+1}
\end{eqnarray*}

\tcb{Would we have expected this to be 0?}

%-------------------------------------

\newpage 
\subsection{Sampling from the dist'n for $\beta$ 
by inverting a Generating Function}
We do not recognize the MGF eq'n \ref{eq:MGF.logistic.eta}
nor the CF eq'n \ref{eq:CF.logistic.eta} as
belonging to a  known distribution.  As mentioned
previously there are numerical procedures for
inverting CFs which can yield
probabilities for the underlying generating 
pdf, and then one could use those probabilities
to generate a sample from that pdf. \tcb{And maybe
this is what we will have to do.}  

\tcb{
 However, \textit{it appears to me that} inversion
 from Laplace Transforms may be a more attractive
 alternative. The restriction to the positive
 real numbers of the Laplace Transform led to 
 the specification of the Half-Logistic distribution
 in Section \ref{subsubsec:HalfLogistic}
 and its Laplace Transform (eq'n \ref{eq:Half.Logistic.Laplace.Transform}). 
 What I think needs to be done next is to connect
 the linear model in eq'n \ref{eq:sum.betas}, which
 is ``in theory'' a sum of $p+1$ root logistic
 random variables, use the Half-Logistic Laplace
 Transform to generate samples from the Half-Logistic,
 and then ``full'' Logistic (as described in Section
 \ref{subsubsec:HalfLogistic}, and sum them to
 yield simulate $\eta$, and this then yields a sample
 from the joint prior for the $\beta$'s that induces
 logistic distribution for $\eta$, and subsequently
 induces a Uniform(0,1) distribution for the Bernoulli
 $\theta$.
 }

% \paragraph{Half Logistic.} If $\mu \ge 0$ is the
% logistic location parameter, then define the Half Logistic
% pdf as follows:
% \begin{align*}
% p(x; \mu, s) & =  \frac{2 \exp \left ( -\frac{(x-\mu)}{s} \right )}
% {s \left ( 1+\exp \left ( -\frac{(x-\mu)}{s}\right )
% \right )^2}, ~~ x \ge \mu 
% \end{align*}
% Based on an integral 
% calculator\footnote{https://www.integral-calculator.com/},
% this integrates to 1 on ($\mu, \infty$) but the expected 
% value, $E_X[X]$ does not exist (the integral is divergent). The MGF $E_X[\exp(tX)]$, integrated over
% ($\mu, \infty$), diverges for some
% values of $t$ but numerical approximations can be found
% with relatively small $t$, e.g., $t$=0.01.

% However, ``it appears'' (based on the integral calculator)
% that Laplace transform can be evaluated, i.e.
% \begin{align*}
% E_X[\exp(-tX)] & = \int_{\mu}^\infty \exp(-tx) \frac{2 \exp \left ( -\frac{(x-\mu)}{s} \right )}
% {s \left ( 1+\exp \left ( -\frac{(x-\mu)}{s}\right )
% \right )^2} dx < \infty 
% \end{align*}
% However, whether or not an analytical expression results
% appears to be a function of the value of $t$ and $s$,
% and possibly $\mu$.  For example, with $\mu$=0, $s$=4,
% and $t$=1, $E_X[\exp(-tX)]$ = $(-24 \ln(2) - 17)/3$ = 0.1215,
% but if $t$ is changed to 1.2, only a numerical approximation is found, 0.102074.

\newpage 
\subsection{With covariates $\ne$ 1}
We return to the more general, and realistic case
where $\eta$ is a linear combination of $\beta_0$
and the $\beta_i x_i$'s. Assuming the same prior 
 for $\beta_0$ and the $\beta_i x_i$'s, then
we'd have the same situation shown above (eq'n \ref{eq:CF.logistic.eta}).

\tcb{Very speculative:} A slightly more realistic alternative would be
to specify an arbitrary distribution for the intercept 
$\beta_0$ while assuming that the priors for the
partial slope coefficients, $\beta_i$, $i=1,\ldots,p$
are the same (and independent), while 
conditioning on the covariate values, and then ``solving'' for the priors for the $\beta_i$'s.
Something like:
\begin{align*}
  CF(\eta) &= CF(\beta_0 + \sum_{i=1}^p \beta_i x_i)  
  =  CF(\beta_0) \prod_{i=1}^p CF(\beta_i x_i) \\
& \Rightarrow \\
\prod_{i=1}^p CF(\beta_i x_i) &= \frac{CF(\eta)}{CF(\beta_0)} \\
& \Rightarrow \\
CF(\beta_i x_i) &= \left [ \frac{CF(\eta)}{CF(\beta_0)} \right ]^{\frac{1}{p}}
\end{align*}
\tcb{\textbf{Q2: Does this kind of algebraic manipulation of characteristic functions (Fourier
transforms) make any sense?  Have precedence in
other problems? }}

\subsection{CFs for products of random variables}
Consider the product of independent of random 
variables, i.e., $\gamma$=$\beta_i x_i$ combination.

\tcb{\textbf{Q3: Are there are ``useful'' results
for Fourier Transforms of products of independent
random variables?}}
\begin{align*}
CV(\gamma) = CF(\beta x) &= E[e^{it \beta x}] 
= \int e^{it \beta x} \pi(\beta) d\beta 
\end{align*}
\tcb{\textbf{Q4:If conditioned on $x$, treating it as a constant,
then does one end up with a ``scaled'' version of a CF?}}
